# Supplementary material for: SNAP: Efficient Extraction of Private Properties with Poisoning
Source: arXiv:2208.12348 source file (2023-06-21)
Supplement: Supplementary file 1 [file Appendix_Methodology.tex]

\section{Detailed Methodology} \label{apndx:Methodology}

\begin{algorithm*}[h]
	\begin{algorithmic}
		\smallskip
		\State {\bf Input} \begin{description}
			\item[--] $f:$ Target Property
			\item[--] $D_p:$  Poisoned dataset generated using Algorithm \ref{alg:prop_poison}.
			\item[--]  $\fm_p:$  Black-box model trained by the model owner on  dataset  which  includes $D_p$ as a subset. 
			\item[--]  $\mt{0}, ~\mt{1}:$  Possible number  of samples  satisfying target property $f$, where  $m_{t_0} < m_{t_1}$. 
			\item[--]  $\mathcal{D}_f:$ Sampling oracle to distribution of instances with target property $f$.
	%		\item[--] $\threshold:$ Logit threshold.
			\item[--] $q:$ Number of queries.
			\item[--] $v:$ Victim class

		\end{description}
	
		\State {\bf Offline Phase} \begin{description}
			
			\item[--] Sample  instances from $ \mathcal{D}_f$  and  construct datasets $D_0 = \{(\vx_1,y_1),\ldots,(\vx_\mt{0},y_\mt{0}) \}$ and	 $D_1 = \{(\vx_1,y_1),\ldots,(\vx_\mt{1},y_\mt{1}) \}$.
			
			\item[--] Train local models $\fm_0 $ and  $\fm_1$ on datasets $D_0 \cup D_p$ and $D_1 \cup D_p$ respectively.
			
			\item[--] Sample  instances from $ \mathcal{D}_f$  and only retain  samples of  victim class `$v$' i.e., construct dataset $D_{test} = \{(\vx_1,v),\ldots,(\vx_q,v) \}$, such that  $|D_{test}| = q$.
			
			\item[--] Query  $D_{test}$ on $\fm_0$ and $\fm_1$ to obtain set of output probability vectors  $S_0 = \{{\bf o}_1, \ldots,{\bf o}_q \}$ and  $S_1 = \{{\bf o}'_1, \ldots,{\bf o}'_q \}$ respectively, where ${\bf o}_i(c)$ and ${\bf o}'_i(c)$ denotes the output probability given by $\fm_0$ and $\fm_1$ for  class label $c$ on input $\vx_i$. 
			
			\item[--]  Compute  logit values $W_0 = \{w_1, \ldots,w_q \}$ and $W_1 = \{w'_1, \ldots,w'_q \}$, where $w_i = \log({{\bf o}_i(v)}/\sum_{j\neq v} {\bf o}_i(j))$ and $w'_i = \log({{\bf o}'_i(v)}/\sum_{j\neq v} {\bf o}'_i(j))$.
			
			\item[--] Fit  pair of  Gaussians $X_{\world{0}}\sim(\mu_{\world{0}},\sigma_{\world{0}})$ and $X_{\world{1}}\sim(\mu_{\world{1}},\sigma_{\world{1}})$ on logit values $W_0$ and $W_1$ respectively and  compute threshold $\threshold$ using theorem \ref{thm:thresholdcomp}.
		
	\end{description}
		
	\State {\bf Online Phase} \begin{description}
		
		\item[--] Query $\mathcal{M}_p$ on $D_{test}$, obtain  a set of output probability vectors and compute the logit values $W_{test}$, similar to  $W_0$ and $W_1$.
		
		\item[--]Check  if  greater than $q/2$ values in set $W_{test}$ satisfy $w_i < \threshold$, then set $b = 0$ else  set $b = 1$.
	\end{description}

	\State \Return $b$,  where  bit $b$ indicates whether $t_b = t_0$ or $t_b = t_1$.
	\end{algorithmic}
	\caption{Detailed Strategy of our attack}
	\label{alg:blackbox}
\end{algorithm*}
